# Supplementary material for: Kondo Insulator to Semimetal Transformation Tuned by Spin-Orbit Coupling
Source: arXiv:1612.03972 source file (2017-06-16)
Supplement: Supplementary file 1 [file SM_final.pdf]

# Supplemental Material of "Kondo insulator to semimetal transformation tuned by spin-orbit coupling "

S. Dzsaber, L. Prochaska, A. Sidorenko, G. Eguchi, R. Svagera, M. Waas, A. Prokofiev, Q. Si, and S. Paschen

## I. METHODS

$Ce_3Bi_4(Pt_{1-x}Pd_x)_3$ single crystals were grown using a modified Bi flux method, described in detail below (Sect. II). Powder X-ray diffraction (XRD) measurements were performed on all grown crystals with a commercial X-ray powder diffractometer (PANalytical XPert Pro MPD), using $CuK_\alpha$ radiation (1.54056 Å). A few mg of representative crystals were selected under an optical microscope, and powdered on a Si single crystal wafer oriented in the [007] crystallographic direction, to avoid any reflection of the substrate. The chemical composition and the Pd substitution levels were determined using energy dispersive X-ray (EDX) and wavelength dispersive X-ray (WDX) spectroscopy setups mounted on a commercial scanning electron microscope (SEM: Philips XL-30, EDX: EDAX New XL-20 135-10 UTW+detector, WDX: Microspec WDX-600). The electrical resistivity of the samples was measured using the standard 4-point method, and contacts were made using conductive silver paint. The samples with $x = 0$ and 0.08 were measured in a Quantum Design PPMS, the samples with $x = 0.18$, 0.37, and 1 were measured in a standard $^4$He flow cryostat, using a lock-in amplifier with an excitation of 100 $\mu$A at a frequency of 33.864 Hz. Crystals with similar shape and size were measured. The magnetic susceptibility was measured using a commercial Cryogenic DC SQUID magnetometer at 100 mT and a Quantum Design PPMS VSM option for the $x = 1$ sample. Measurements below 2 K were performed with a $^3$He insert of the DC SQUID magnetometer. For the $x = 0.37$ crystal, a field of 7 T had to be applied to obtain a good signal. This does not strongly affect the susceptibility in view of the nearly linear-in-$B$ magnetization at 2 K [Fig. 4(c) main part]. Also the $M(B)$ isotherms for the $x = 1$ sample at 2 and 0.7 K are only weakly nonlinear [Fig. 4(c) main part]. The magnetic property measurements were performed on the same crystals selected for the resistivity measurements, except for $x = 1$, where 14 representative crystals where measured simultaneously to enhance the resolution. The specific heat measurements in zero field and at 7 T for the $x = 1$ sample

were done in a $^4$He Quantum design PPMS system using the thermal relaxation method. In zero field, these measurements were extended to lower temperatures using a $^3$He insert of a Quantum design PPMS system. To enhance the resolution, the same 14 crystals as used for the magnetic characterization were measured simultaneously.

## II. CRYSTAL GROWTH

Five $Ce_3Bi_4(Pt_{1-x}Pd_x)_3$ crystals with the nominal substitution levels $x_n = 0$, 0.1, 0.15, 0.3, and 1 were grown using the Bi flux technique [1]. The actual substitution levels $x$ where determined by EDX measurements, as described below (Sect. III). For $x_n = 0$ and 0.1, elementary Ce, Pt, Pd, and Bi in an atomic ratio of $1 : 1 - x_n : x_n : 7$, respectively, were placed in an alumina crucible, and heated to 1100°C in a vacuum sealed quartz tube, using a box furnace. The melt was then slowly cooled to 600°C with a cooling rate of 1°C/h and left annealing for 12 h. Crystals of typically 1 mm diameter were then extracted from the melt using a centrifuge. We found that this method is not adequate for growing the Pd substituted crystals with $x > 0.1$, as therein the primary stable phase at Bi excess is $CeBi_2Pd$ [2]. For Pd substituted samples with $x > 0.1$, a premelt of $CePt_{1-x}Pd_x$ was prepared by melting a stoichiometric amount of the elementary materials in an RF induction furnace under Ar atmosphere. The premelt was then placed in an alumina crucible with Bi in a vacuum sealed quartz tube, and the same heat treatment and growth rates were applied as in case of $x = 0$. We found that the ratio Ce:Pt:Pd:Bi of $1 : 1 - x_n : x_n : 1.5$ is the optimum to grow Pd substituted crystals. This optimum ratio comes from the interplay of two effects: A smaller content of Bi results in an increased melting temperature of the compound and a quick depletion of the Bi flux (as it is already close to the stoichiometric ratio of $1 : 1 : 1.33$ of the Pd free material), thus impeding the growth of the crystals. However, if the Bi content is higher, a considerable amount of $CeBi_2Pd$ is detected in the XRD diffractogram. The unavoidable quick depletion of the Bi flux limits the size of the grown crystals to diameters of about 300 $\mu$m.

## III. STRUCTURAL AND CHEMICAL ANALYSES

The $Ce_3Bi_4(Pt_{1-x}Pd_x)_3$ compounds crystallize in the cubic $Y_3Sb_4Au_3$ phase of space group $I\bar{4}3d$, as evidenced by the powder XRD measurements (Fig. S1). The unit cell ($a =$ 10.051 Å for $Ce_3Bi_4Pt_3$, $a = 10.058$ Å for $Ce_3Bi_4Pd_3$) contains 4 formula units. Thus, 40 atoms make up the rather complicated structure. To better capture it, the local environment of the Ce atom – which is most essential in shaping the extraordinary physical properties of the compound – is presented in its position in the unit cell (lower right inset of Fig. 3, main text) and alone, emphasizing the Pt positions (upper right inset of Fig. 3, main text). Each Ce atom is surrounded by 12 atoms (4 Pt/Pd and 8 Bi). However, Ce has only Pd/Pt atoms as nearest neighbors at 3.01 Å distance, arranged in a tetrahedral configuration. The second nearest neighbors are formed by 8 Bi atoms in a distorted polyhedral structure, at a distance of 3.41 Å. The crystal structure and peak positions deduced from the XRD diffractograms for $x = 0$ and 1 are in good agreement with the previously reported structures of $Ce_3Bi_4Pt_3$ [3] and $Ce_3Bi_4Pd_3$ [4], respectively. The diffraction patterns for $0 \geq x > 1$ show a minor Bi peak, that is due to incomplete centrifuging.

EDX results are presented in Fig. S2 in the range of 0.5 keV to 3.5 keV where the strongest Pt-$M$, Bi-$M$, and Pd-$L$ peaks are located at 2 keV, 2.5 keV, and 2.9 keV, respectively. The Pd substitution levels were determined from these spectra. They follow the trend of the nominal substitution levels [Fig. S2(a, inset)]. For unsubstituted $Ce_3Bi_4Pt_3$, the Pt-$M$ peak is comparable in height with the Bi-$M$ peak, whereas the Pd-$L$ lines are absent [Fig. S2(a), black curve]. With increasing Pd substitution, the height of the Pt-$M$ peak successively decreases, and that of the Pd-$L$ peaks increases, while the sum of the atomic contents is unchanged [Fig. S2(a) inset]. This proves that Pd indeed substitutes Pt at the Pt sites of $Ce_3Bi_4Pt_3$, and does not form a separate phase. An SEM image of a selected crystal with $x =$ 0.37 [Fig. S2(b)] shows that the substitution is homogeneous and that no secondary phases are present on the sample surface. For the $x = 0.08$ sample, the nominal total Pd atomic content is 2.4 at%, which is comparable to the lower detection limit of the EDX technique. To improve the detection limit, the crystal was also investigated by WDX spectroscopy, which has a better energy resolution, and confirms the presence of a small amount of Pd in the $x = 0.08$ sample [Fig. S2(c)].

## IV. SPECIFIC HEAT AND MAGNETIC SUSCEPTIBILITY OF $CE_3BI_4PD_3$ BELOW 2 K

To explore the physics at very low energies, we have extended our measurements of the specific heat and magnetic susceptibility to below 2 K. Our results uncover additional signs of strong correlations. The electronic specific heat coefficient $C_{el}/T$ of $Ce_3Bi_4Pd_3$ shows a Schottky-like anomaly and an $\ln(1/T)$ upturn below 2 and 0.8 K, respectively (Fig. S3, left axis). An $\ln(1/T)$ upturn is also seen in the magnetic susceptibility $\chi(T)$ data (Fig. S3, right axis), but the Schottky-like anomaly is absent here.

Let us first consider the Schottky-like anomaly. Because it appears in the specific heat but not in the magnetic response, it can be attributed to charge as opposed to spin excitations. Thus, this anomaly is likely a precursor to the formation of a charge density wave (CDW). Indeed, among the various competing orders that may develop out of a Weyl semimetal, long-range repulsive Coulomb interactions enhance the tendency towards a CDW at the wavevector that connects the Weyl nodes [5].

Next we discuss the $\ln(1/T)$ feature. Given that it appears in both the specific heat and the magnetic susceptibility, it likely reflects the physics in the spin sector. In metallic heavy fermion systems with regular Fermi surfaces, logarithmic divergences are a hallmark of non-Fermi liquid behavior [6, 7], which is often associated with quantum criticality. In most Weyl semimetals, the Weyl nodes are not exactly situated at the Fermi energy. Assuming this is also the case for $Ce_3Bi_4Pd_3$, the RKKY interaction in this heavy fermion system can compete against the Kondo coupling and give rise to a nearby magnetic quantum critical point. This is consistent with the fact that the logarithmic dependence is only discernible at temperatures that are low compared even to the Kondo temperature. It is worth noting that similar logarithmic behavior at low temperatures has recently been observed in another heavy fermion semimetal, namely $CeNi_{2-\delta}As_2$ under pressure [8].

To ascertain the internal consistency of the picture we have proposed, we have analyzed the specific heat by subtracting the Schottky-like anomaly and the $\ln(1/T)$ upturn from the $C_{el}/T$ data. We find that the linear-in-$T^2$ behavior persists down to the lowest measured temperature, 0.4 K [Fig. S3 and Fig. 5(d) of main part]. This result is significant in two ways. First, it extends the dynamical range for the signature of the nodal excitations of a Weyl-Kondo semimetal [9]: The linear-in-$T^2$ component in $C_{el}/T$ now occurs over more than

a decade in temperature, from 0.4 to 5.5 K. Second, it provides evidence that the Weyl nodes in $Ce_3Bi_4Pd_3$ are located remarkably close to the Fermi energy. The hallmark tunability of heavy fermion systems implies that $Ce_3Bi_4Pd_3$ is an ideal system in which the Weyl nodes can be further tuned, by e.g. pressure or magnetic field, to lie exactly at the Fermi energy.

We close by noting that the very low-temperature features described above are of great interest on their own and certainly motivate further studies. They show that the presence of strong spin-orbit coupling enriches the global phase diagram of heavy fermion materials [7, 10]. The great tunability of these systems, including the controlled variation of spin-orbit coupling newly demonstrated here, raises the prospect of new phases – such as the aforementioned CDW whose ordering wavevector retains information about the Weyl nodes – emerging in the overall phase diagram of $Ce_3Bi_4Pd_3$ and a variety of other Kondo semimetals.

---


[1] P. C. Canfield and Z. Fisk, Philos. Mag. B **65**, 1117 (1992).

[2] F. Han, X. Wan, D. Phelan, C. C. Stoumpos, M. Sturza, C. D. Malliakas, Q. Li, T.-H. Han, Q. Zhao, D. Y. Chung, and M. G. Kanatzidis, Phys. Rev. B **92**, 045112 (2015).

[3] M. F. Hundley, P. C. Canfield, J. D. Thompson, Z. Fisk, and J. M. Lawrence, Phys. Rev. B **42**, 6842 (1990).

[4] W. Hermes, S. Linsinger, R. Mishra, and R. Pöttgen, Monatsh. Chem. **139**, 1143 (2008).

[5] H. Wei, S.-P. Chao, and V. Aji, Phys. Rev. B **89**, 235109 (2014).

[6] H. v. Löhneysen, A. Rosch, M. Vojta, and P. Wölfle, Rev. Mod. Phys. **79**, 1015 (2007).

[7] Q. Si and S. Paschen, Phys. Status Solidi B **250**, 425 (2013).

[8] Y. Luo, F. Ronning, N. Wakeham, X. Lu, T. Park, Z.-A. Xu, and J. D. Thompson, Proc. Natl. Acad. Sci. USA **112**, 13520 (2015).

[9] H.-H. Lai, S. E. Grefe, S. Paschen, and Q. Si, Weyl-Kondo semimetal in a heavy fermion system, arXiv:1612.03899v1, 2016.

[10] J. Custers, K. Lorenzer, M. Müller, A. Prokofiev, A. Sidorenko, H. Winkler, A. M. Strydom, Y. Shimura, T. Sakakibara, R. Yu, Q. Si, and S. Paschen, Nature Mater. **11**, 189 (2012).

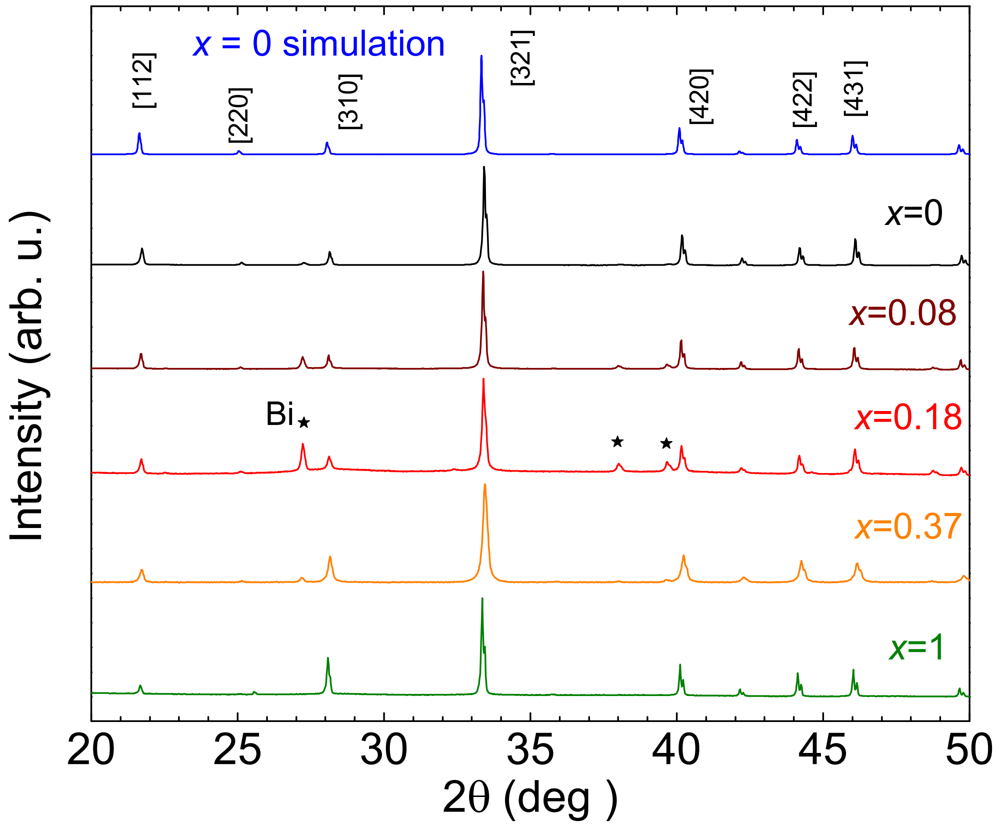


FIG. S1. (Color online) Powder XRD patters of all investigated batches. The Miller indices and XRD simulation of $Ce_3Bi_4Pt_3$ are also shown. Minor peaks from remaining Bi flux are observed and indicated by stars. They are absent in $Ce_3Bi_4Pd_3$.

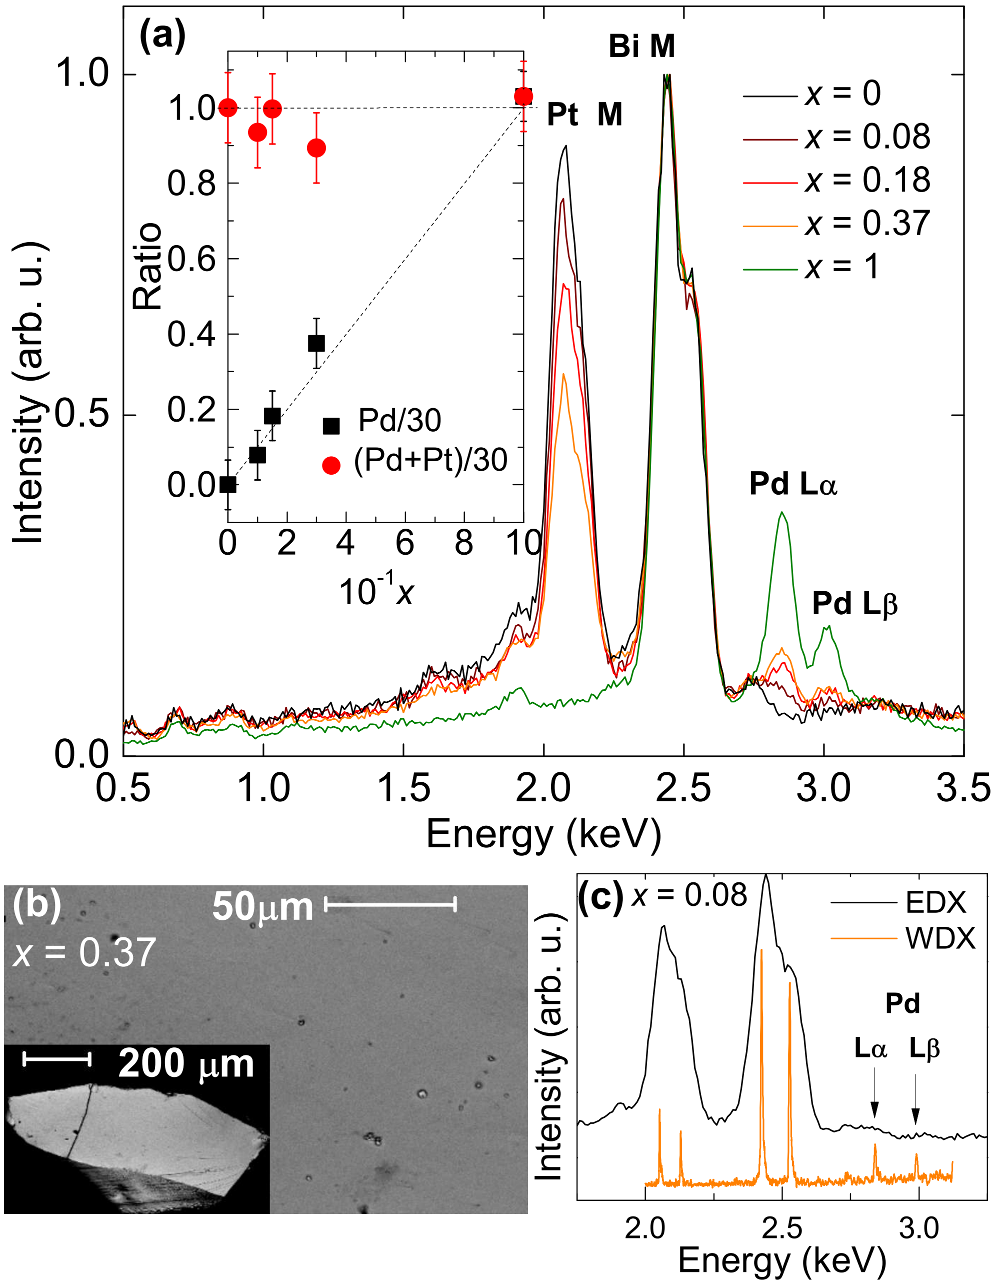


FIG. S2. (Color online) SEM, EDX, and WDX study of $Ce_3Bi_4(Pt_{1-x}Pd_x)_3$. (a) Variation of the EDX spectra as function of the substitution level (normalized to the Bi-$M$ peak). The inset shows the Pd content along with the Pd+Pt content as compared to the nominal values (dashed lines). (b) Representative SEM image of a $x = 0.37$ sample. (c) WDX spectrum of the $x = 0.08$ sample with clearly resolved Pd peaks.

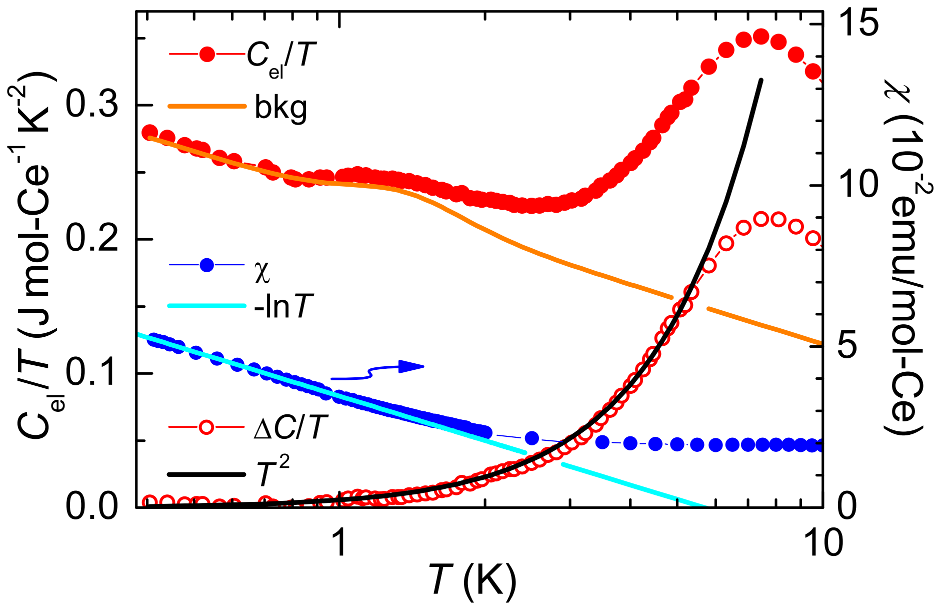


FIG. S 3. (Color online) Electronic specific heat coefficient $C_{\rm el}/T$ (left axis) and magnetic susceptibility $\chi$ (right axis) of $Ce_3Bi_4Pd_3$ plotted vs $\log T$ between 0.4 and 10 K. The orange line describes a Schottky-like anomaly below 2 K, residing on top of an $\ln(1/T)$ upturn, – signatures of a precursor to the formation of a charge density wave and of quantum criticality, respectively (see text). As such they represent an electronic "background" (bkg) to the linear-in-$T^2$ contribution of a Weyl-Kondo semimetal ($\Delta C/T = C_{\rm el}/T -$ bkg, black line represents $T^2$ fit), that extends from 5.5 K to the lowest temperatures. The corresponding quasiparticle velocity $v^*$ [9] is, with 870 m/s, comparable to the value of 885 m/s determined without background subtraction (see main text). The magnetic susceptibility shows the $\ln(1/T)$ behavior, but lacks the Schottky-like anomaly, suggesting that the anomaly involves charge as opposed to spin excitations.
